# Supplementary material for: Topology-Aware Differential Privacy in Hierarchical Federated Learning
Source: arXiv:2506.19260 source file (2026-08-19)
Supplement: Supplementary file 1 [file appendix.tex]

%% Fulcrum — Supplementary Material
%% Proofs of Theorem V.2 and Theorem V.3

\documentclass[letterpaper,journal]{IEEEtran}

% --- Math ---
\usepackage{amsmath,amsfonts,amssymb}
\usepackage{amsthm}

% --- Typography ---
\usepackage{microtype}

% --- References ---
\usepackage{cite}

% --- Other ---
\usepackage{xspace}
\usepackage{hyperref}

% --- Unnumbered theorem environments for restated results ---
\newtheorem*{theoremstar}{Theorem}
\newtheorem*{corollarystar}{Corollary}

% --- Numbered environments for new lemmas in supplementary ---
\newtheorem{lemma}{Lemma}[section]

% --- Counter continuations from main paper ---
% Last equation in main paper: (5)
% Last figure in main paper: Fig. 6
% Last table in main paper: Table II
\setcounter{equation}{5}
\setcounter{figure}{6}
\setcounter{table}{2}

% --- Macros (must match main paper) ---

\newcommand{\KL}{D_{\mathrm{KL}}}
\newcommand{\FAM}{\mathcal{F}}
\newcommand{\TOPO}{\mathcal{G}}
\newcommand{\Tmax}{T_{\max}}

\begin{document}

\title{Supplementary Material:\\
Topology-Aware Differential Privacy in Federated Learning}

\maketitle

\noindent This supplementary material provides full proofs of Theorem~V.2
and Theorem~V.3 from the main paper. All equation, figure, and
table numbering continues consecutively from the main paper.
Lemmas introduced here are local to this document and are not
referenced in the main text.

\appendix

% =============================================================================
\section{Proof of Theorem~V.2}
\label{app:thm1}
% =============================================================================

\subsection{Statement}

\begin{theoremstar}[V.2 \textnormal{---} Per-client conditional
MI bound]
Under (IA1) and (IA2) from the main paper, for any deterministic
adversary strategy $f$, any prior $\mathbb{P} \in
\FAM_{\TOPO,\omega}$, and any client $i$:
\begin{equation}
I_{\mathbb{P}}\!\left(p_i;\,\hat{p}_i \;\middle|\;
\TOPO,\,\omega,\,\{\sigma_j\}\right)
\;\leq\;
\underbrace{\frac{\Tmax}{2\sigma_i^2\,|B|^2}}_{\text{controllable}}
\;+\;
\underbrace{\ell_i^\circ}_{\text{uncontrollable}}.
\label{eq:thm1-supp}
\end{equation}
\end{theoremstar}

\subsection{Proof Structure}

\noindent The proof decomposes into four lemmas, assembled in
Section~\ref{sec:assembly1}.

\begin{itemize}
\item Lemmas~\ref{lem:chain} and~\ref{lem:lateral} isolate the
      \emph{uncontrollable} lateral-leakage term via a chain-rule
      inequality and the definition of structural leverage.
\item Lemmas~\ref{lem:perround} and~\ref{lem:composition} bound
      the \emph{controllable} mechanism term using the Gaussian
      noise structure of DP-SGD.\medskip
\end{itemize}

\noindent Three standard tools are used throughout: the chain rule of
mutual information and the data processing inequality;
Mironov's RDP composition for the Gaussian
mechanism~\cite{mironov2017rdp}; and the Cuff-Yu max-KL to
MI-DP conversion~\cite{cuff2016mi}.

\subsection{Lemmas}

\begin{lemma}[Chain-rule decomposition]
\label{lem:chain}
For any random variables $X$, $Y$, $Z$:
\[
I(X;\,Y) \;\leq\; I(X;\,Z) \;+\; I(X;\,Y \mid Z).
\]
\end{lemma}

\begin{proof}
By the MI conditioning identity:
\[
I(X;Y) \;=\; I(X;Z) \;+\; I(X;Y \mid Z) \;-\; I(X;Z \mid Y).
\]
The result follows since $I(X;Z \mid Y) \geq 0$.
\end{proof}

\begin{lemma}[Per-round Gaussian-mechanism KL bound]
\label{lem:perround}
Under (IA1) and (IA2), for each round $t$, any $D_{-i}$, and
any adjacent databases $D_i$, $D_i'$:
\begin{equation}
\KL\!\left(
\mathbb{P}_{\theta_i^{(t)} \mid D_i,\, \theta^{(t-1)},\, D_{-i}}
\;\Big\|\;
\mathbb{P}_{\theta_i^{(t)} \mid D_i',\, \theta^{(t-1)},\,
D_{-i}}\right)
\;\leq\;
\frac{1}{2\sigma_i^2\,|B|^2}.
\label{eq:kl-bound}
\end{equation}
Consequently, by the Cuff-Yu conversion~\cite{cuff2016mi}:
\[
I\!\left(D_i;\;\theta_i^{(t)} \;\middle|\;
\theta^{(t-1)},\,D_{-i}\right)
\;\leq\; \frac{1}{2\sigma_i^2\,|B|^2}.
\]
\end{lemma}

\begin{proof}
Conditional on $\theta^{(t-1)}$ and $D_{-i}$, the round-$t$
update (Eq.~(1) of the main paper) applies the Gaussian
mechanism to the per-sample average of clipped gradients
of $D_i$.

\medskip
\noindent\textit{Sensitivity.} Each clipped gradient has norm
at most $C$, so the sensitivity of the averaged gradient is:
\[
\Delta \;=\; \frac{C}{|B|}.
\]

\noindent\textit{Noise scale.} The per-round noise is
$\xi_i^{(t)} \sim \mathcal{N}(0, \sigma_i^2 C^2 I)$, giving
effective noise scale $s = \sigma_i C$ on the averaged gradient,
where $\sigma_i > 0$ is the dimensionless multiplier of Abadi
et~al.~\cite{abadi2016dpsgd}.

\medskip
\noindent\textit{KL bound.} The KL divergence between adjacent
mechanism outputs is:
\[
\frac{\Delta^2}{2s^2}
\;=\; \frac{(C/|B|)^2}{2(\sigma_i C)^2}
\;=\; \frac{C^2/|B|^2}{2\sigma_i^2 C^2}
\;=\; \frac{1}{2\sigma_i^2\,|B|^2},
\]
establishing~\eqref{eq:kl-bound}. The Cuff-Yu max-KL
bound~\cite{cuff2016mi} then implies MI-DP with the same
parameter, giving the stated MI inequality.
\end{proof}

\begin{lemma}[Sequential composition]
\label{lem:composition}
Under (IA1) and (IA2), sequential composition of the per-round
bound across all $\Tmax$ rounds gives:
\begin{align*}
I\!\left(D_i;\;\Theta_i \;\middle|\; D_{-i}\right)
&\;\leq\;
\sum_{t=1}^{\Tmax}
I\!\left(D_i;\;\theta_i^{(t)} \;\middle|\;
\theta^{(t-1)},\,D_{-i}\right) \\
&\;\leq\;
\frac{\Tmax}{2\sigma_i^2\,|B|^2}.
\end{align*}
\end{lemma}

\begin{proof}
\textit{Step 1: Chain rule.} By the MI chain rule:
\[
I(D_i;\Theta_i \mid D_{-i})
\;=\; \sum_{t=1}^{\Tmax}
I\!\left(D_i;\;\theta_i^{(t)} \;\middle|\;
\theta_i^{(<t)},\,D_{-i}\right).
\]

\noindent\textit{Step 2: Conditioning inequality.}
For each term, we claim:
\[
I\!\left(D_i;\;\theta_i^{(t)} \;\middle|\;
\theta_i^{(<t)},\,D_{-i}\right)
\;\leq\;
I\!\left(D_i;\;\theta_i^{(t)} \;\middle|\;
\theta^{(t-1)},\,D_{-i}\right).
\]
To see this, note that conditional on $D_{-i}$ and
$\theta_i^{(<t)}$, the global state $\theta^{(t-1)}$ is a
deterministic function of $\theta_i^{(<t)}$,
$\Theta_{-i}^{(<t)}$, and the aggregation rule. Since
$\Theta_{-i}^{(<t)}$ depends only on $D_{-i}$ and noise
$\{\xi_j^{(<t)}\}_{j \neq i}$, which is independent of $D_i$
by (IA1) and (IA2), $\theta^{(t-1)}$ is conditionally
independent of $D_i$ given $(\theta_i^{(<t)}, D_{-i})$.
The Markov chain
\[
D_i \;\longrightarrow\; \theta_i^{(<t)}
\;\longrightarrow\;
\bigl(\theta_i^{(<t)},\,\theta^{(t-1)}\bigr)
\]
and the data processing inequality therefore imply that
conditioning additionally on $\theta^{(t-1)}$ cannot increase
the MI.

\medskip
\noindent\textit{Step 3: Apply Lemma~\ref{lem:perround}.}
Each term is bounded by $1/(2\sigma_i^2|B|^2)$. Summing
over $t = 1, \ldots, \Tmax$ completes the proof.
\end{proof}

\begin{lemma}[Lateral-leakage bound]
\label{lem:lateral}
Under (IA2):
\[
I\!\left(p_i;\;D_{-i}\right) \;\leq\; \ell_i^\circ.
\]
\end{lemma}

\begin{proof}
Immediate from Definition~V.1 of the main paper, which defines
$\ell_i^\circ$ as $\sup_{\mathbb{P} \in \FAM_{\TOPO,\omega}}
I_{\mathbb{P}}(p_i; D_{-i})$.
\end{proof}

\subsection{Assembly}
\label{sec:assembly1}

We now combine the four lemmas. Let $(\cdot)$ denote
conditioning on $(\TOPO, \omega, \{\sigma_j\})$ throughout;
these are deployment constants, not random variables.

\medskip
\noindent\textit{Step 1 (data processing).}
Since $\hat{p}_i = f(\Theta)$ is a deterministic function of
the observations:
\[
I(p_i;\,\hat{p}_i \mid \cdot)
\;\leq\; I(p_i;\,\Theta \mid \cdot).
\]

\noindent\textit{Step 2 (chain rule).}
Applying Lemma~\ref{lem:chain} with $X = p_i$, $Y = \Theta$,
$Z = D_{-i}$:
\[
I(p_i;\,\Theta \mid \cdot)
\;\leq\;
I(p_i;\,D_{-i})
\;+\; I(p_i;\,\Theta \mid D_{-i}).
\]

\noindent\textit{Step 3 (lateral term).}
By Lemma~\ref{lem:lateral}:
\[
I(p_i;\,D_{-i}) \;\leq\; \ell_i^\circ.
\]

\noindent\textit{Step 4 (independence of other clients).}
Under (IA1), $\Theta_{-i}$ is independent of $D_i$ given
$D_{-i}$. Therefore:
\[
I(p_i;\,\Theta \mid D_{-i})
\;=\; I(p_i;\,\Theta_i \mid D_{-i}).
\]

\noindent\textit{Step 5 (data processing on $p_i$).}
Since $p_i$ is a deterministic function of $D_i$:
\[
I(p_i;\,\Theta_i \mid D_{-i})
\;\leq\; I(D_i;\,\Theta_i \mid D_{-i}).
\]

\noindent\textit{Step 6 (composition bound).}
By Lemma~\ref{lem:composition}:
\[
I(D_i;\,\Theta_i \mid D_{-i})
\;\leq\; \frac{\Tmax}{2\sigma_i^2\,|B|^2}.
\]

\noindent Chaining Steps 1--6 gives:
\[
I(p_i;\,\hat{p}_i \mid \cdot)
\;\leq\;
\frac{\Tmax}{2\sigma_i^2\,|B|^2}
\;+\; \ell_i^\circ,
\]
which is the statement of Theorem~V.2. \hfill\qed

% =============================================================================
\section{Proof of Theorem~V.3}
\label{app:thm2}
% =============================================================================

\subsection{Statement}

\begin{theoremstar}[V.3 \textnormal{---} Balanced min-max
allocation]
For any utility budget $U > 0$, the unique solution to:
\begin{equation}
\min_{\{\sigma_i^2 > 0\}}\;
\max_i \left[\, \frac{a}{\sigma_i^2} + \ell_i^\circ \,\right]
\quad \text{subject to} \quad
\sum_{i=1}^n \sigma_i^2 \leq U,
\label{eq:opt-supp}
\end{equation}
where $a := \Tmax/(2|B|^2)$, is:
\[
\sigma_i^{*\,2} \;=\; \frac{a}{K^\star - \ell_i^\circ},
\]
where $K^\star$ is the unique solution to:
\begin{equation}
\sum_{i=1}^n \frac{a}{K^\star - \ell_i^\circ} \;=\; U,
\qquad K^\star > \max_i\,\ell_i^\circ.
\label{eq:budget-supp}
\end{equation}
The achieved worst-case per-client MI bound is $K^\star$,
equilibrated uniformly across all clients.
\end{theoremstar}

\subsection{Proof Structure}

\noindent Problem~\eqref{eq:opt-supp} has a non-smooth $\max$ objective.
The proof proceeds in three steps.

\begin{enumerate}
\item \textit{Reformulation.} Introduce a slack variable $K$
      to convert the $\max$ objective into a linear one, yielding
      a convex programme.
\item \textit{Strong duality.} Verify Slater's condition to
      establish that KKT conditions are necessary and sufficient.
\item \textit{KKT analysis.} Derive the closed-form solution
      and establish uniqueness of $K^\star$.
\end{enumerate}

\subsection{Convex Reformulation}

\noindent Introduce slack variable $K$ to rewrite~\eqref{eq:opt-supp}:
\begin{equation}
\min_{K,\,\{\sigma_i^2 > 0\}} K
\quad\text{subject to}\quad
\frac{a}{\sigma_i^2} + \ell_i^\circ \leq K \;\;\forall\, i,
\quad \sum_{i=1}^n \sigma_i^2 \leq U.
\label{eq:opt-reform-supp}
\end{equation}

\noindent The objective is linear in $K$. The per-client constraints are
convex since $a/\sigma_i^2$ is convex and strictly decreasing
on $\sigma_i^2 > 0$. The budget constraint is linear.

\medskip
\noindent\textit{Slater's condition.} Setting $\sigma_i^2 =
U/(2n)$ for all $i$ is strictly feasible, with:
\[
K \;=\; \frac{2na}{U} + \max_i \ell_i^\circ
\;>\; \frac{a}{\sigma_i^2} + \ell_i^\circ
\quad \forall\, i.
\]
Strong duality therefore holds, and KKT conditions are
necessary and sufficient for optimality.

\subsection{KKT Analysis}

\begin{lemma}[KKT optimality]
\label{lem:kkt}
The unique solution to \eqref{eq:opt-reform-supp} satisfies:
\[
\sigma_i^{*\,2} \;=\; \frac{a}{K^\star - \ell_i^\circ}
\quad \forall\, i,
\]
where $K^\star$ is the unique root of
$g(K) = \sum_i a/(K - \ell_i^\circ) = U$ on
$({\max_i \ell_i^\circ},\, \infty)$.
\end{lemma}

\begin{proof}
The Lagrangian for \eqref{eq:opt-reform-supp} is:
\[
\mathcal{L}
\;=\; K
\;+\; \sum_{i=1}^n \mu_i
      \!\left(\frac{a}{\sigma_i^2} + \ell_i^\circ - K\right)
\;+\; \lambda\!\left(\sum_{i=1}^n \sigma_i^2 - U\right),
\]
with multipliers $\mu_i \geq 0$ and $\lambda \geq 0$.

\medskip
\noindent\textit{Stationarity in $K$.}
\[
\frac{\partial \mathcal{L}}{\partial K}
\;=\; 1 - \sum_{i=1}^n \mu_i \;=\; 0
\;\implies\;
\sum_{i=1}^n \mu_i \;=\; 1.
\]

\noindent\textit{Stationarity in $\sigma_i^2$.}
\[
\frac{\partial \mathcal{L}}{\partial \sigma_i^2}
\;=\; -\frac{\mu_i a}{\sigma_i^4} + \lambda \;=\; 0
\;\implies\;
\sigma_i^{*\,2} \;=\; \sqrt{\frac{\mu_i a}{\lambda}}.
\]

\noindent\textit{All constraints are active.}
Suppose the per-client constraint for some $i$ were inactive.
Then $\mu_i = 0$ by complementary slackness. Stationarity
in $\sigma_i^2$ then requires $\lambda = 0$. But $\lambda = 0$
forces $\mu_j = 0$ for all $j$, contradicting $\sum_i \mu_i =
1$. Therefore all per-client constraints are active at the
optimum:
\[
\frac{a}{\sigma_i^{*\,2}} + \ell_i^\circ \;=\; K^\star
\quad \forall\, i,
\]
which gives the closed form
$\sigma_i^{*\,2} = a/(K^\star - \ell_i^\circ)$.

\medskip
\noindent\textit{Uniqueness of $K^\star$.}
Define $g(K) = \sum_i a/(K - \ell_i^\circ)$ on the domain
$(K_{\min}, \infty)$ where $K_{\min} = \max_i \ell_i^\circ$.
Then:
\begin{itemize}
\item $g$ is continuous and strictly decreasing on
      $(K_{\min}, \infty)$,
\item $g(K) \to +\infty$ as $K \downarrow K_{\min}$,
\item $g(K) \to 0$ as $K \to +\infty$.
\end{itemize}
By the intermediate value theorem, for any $U > 0$ there exists
a unique $K^\star \in (K_{\min}, \infty)$ with
$g(K^\star) = U$.
\end{proof}

\subsection{Strict Improvement over Uniform Allocation}

\begin{corollarystar}[V.4 \textnormal{---} Strict improvement
over uniform allocation]
Let $K_{\mathrm{uniform}} = an/U + \max_i \ell_i^\circ$ denote
the worst-case MI bound under uniform allocation
$\sigma_i^2 = U/n$. Then:
\[
K^\star \;\leq\; K_{\mathrm{uniform}},
\]
with equality if and only if all $\ell_i^\circ$ are equal.
\end{corollarystar}

\begin{proof}
Uniform allocation $\sigma_i^2 = U/n$ for all $i$ is feasible
for \eqref{eq:opt-reform-supp} and achieves objective value
$K_{\mathrm{uniform}}$. Since $K^\star$ is the minimum of
\eqref{eq:opt-reform-supp}, we have $K^\star \leq
K_{\mathrm{uniform}}$. Equality holds if and only if uniform allocation satisfies the
KKT conditions of Lemma~\ref{lem:kkt}, which requires:
\[
\frac{a}{U/n} + \ell_i^\circ \;\equiv\; K^\star
\quad \forall\, i.
\]
This holds if and only if all $\ell_i^\circ$ are equal.
\end{proof}

\subsection{Edge Cases and Computational Note}

\noindent\textit{Small utility budget.} The KKT solution
requires $K^\star > \max_i \ell_i^\circ$, which holds for all
$U > 0$ by Lemma~\ref{lem:kkt}. However, when $U$ is very
small, the solution concentrates the budget on high-leverage
clients ($\sigma_i^2 \to 0$ for low-leverage clients), falling
below the practically deployable range for DP-SGD. This regime
is not analysed further.

\medskip
\noindent\textit{Computation.} Solving $g(K^\star) = U$ via
one-dimensional bisection on $K$ requires
$O(n \log(1/\varepsilon))$ operations for tolerance
$\varepsilon$, which is negligible for $n \leq 500$.

\bibliographystyle{IEEEtran}
\bibliography{references}

\end{document}
